# Supplementary material for: Soft self-assembly of Weyl materials for light and sound
Source: arXiv:1711.11019 ancillary file (2018-04-29)
Supplement: Supplementary file 1 [file SI_self_assembled_weyl.pdf]

# Supporting Informations to Soft self-assembly of Weyl materials for light and sound

Michel Fruchart<sup>a,1</sup>, Seung-Yeol Jeon<sup>b</sup>, Kahyun Hur<sup>b</sup>, Vadim Cheianov<sup>a</sup>, Ulrich Wiesner<sup>c</sup>, and Vincenzo Vitelli<sup>a,d,2</sup>

<sup>a</sup>Lorentz Institute, Leiden University, Leiden 2300 RA, The Netherlands; <sup>b</sup>Center for Computational Science, Korea Institute of Science and Technology, Seoul 02792, Republic of Korea; <sup>c</sup>Department of Materials Science and Engineering, Cornell University, Ithaca, New York 14850, USA.; <sup>d</sup>Department of Physics, The University of Chicago, Chicago, IL 60637, USA.

**Code and data availability.** The code used to compute the photonic band structures, the charges of the Weyl points, the irreducible representations of the numerical eigenvectors, the space group of the structures and the spectra of the effective Hamiltonians is available on the Zenodo repository <https://doi.org/10.5281/zenodo.1182581>. The code used to compute the dispersive photonic, elastic and acoustic band structures can be obtained on request.

**Determination of the space groups.** Computing a space group is generally tedious and error prone. To automatize the procedure, we reduce the structure to a set of points having the same space group, which can be processed by the open-source library spglib (1). Following Schoen (2), we consider the *skeletal graph* associated to a (single) gyroid surface, which can be thought as the limit of an infinitely contracted gyroid (see figure 1). To be concrete, this skeletal graph  $\Gamma_+$  has three-coordinated vertices located at each of the 8 Wyckoff positions with label “a” of the space group  $I4_132$  (IUC 214) [see e.g. (3) or (4)], which correspond to the global maxima of the function  $g$  defining the isosurface in paragraph *Self-assembling inversion-asymmetric gyroids* of the main text. The enantiomeric partner  $\Gamma_-$  of this skeletal graph is obtained by space inversion with respect to the point  $(1/2, 1/2, 1/2)$ . While a single of such skeletal graphs describes, from the point of view of space group symmetry, the single gyroid structure, their union describes either the asymmetric double gyroid or the symmetric double gyroid, depending on whether the points in  $\Gamma_{\pm}$  are colored differently or not. The results of the symmetry analysis is summarized in table 1 and, indeed, reproduce the well-known results about the single and double gyroid structures. Such a tool becomes useful when the structure is modified, for example by strain: applying the strain matrix to the positions of the nodes of  $\Gamma_{\pm}$  gives a new skeletal graph. The space group of this graph (and of the corresponding strained structure) can then be determined in the same way, as exemplified for the shear strain defined in the main text in table 1. Similarly, the presence of air spheres such as in references (5–7) can be described from the point of view of symmetries by the addition of new nodes in the graph, colored differently from all the other ones.

**Determination of the irreducible representations at  $\Gamma$ .** The aim of this section is to compute the representation along which the numerical eigenvectors transform, and to decompose it on the basis of irreducible representations. For our analysis to hold, it is crucial that the three-fold degeneracy at the  $\Gamma$  point be an essential degeneracy (due to the octahedral symmetry), and not an accidental degeneracy which could arise from a fine tuning of the system parameters. To ensure that it is indeed the case from the numerical eigenfrequencies is not straightforward: one has to perturb the system to verify that

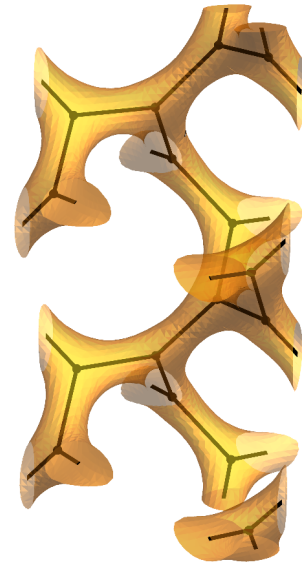

**Fig. 1. Skeletal graph of a single gyroid.** We show two repetitions of a (non-primitive) cubic cell of a single gyroid, along with the associated skeletal graph (in black).

the degeneracy is stable, and one has to take into account that the degeneracy is effectively lifted by numerical errors. A more reliable way is to study the effect of symmetry operations on the eigenvectors: the set of  $g$  eigenvectors involved in an essential degeneracy should transform along a single  $g$ -dimensional irreducible representation.

Although the space group  $Ia\bar{3}d$  (IUC 230) of the double gyroid is nonsymmorphic, the  $\Gamma$  point is not on the Brillouin zone boundary, and the irreducible representations of the space

| structure       | space group            | point group at $\Gamma$ |
|-----------------|------------------------|-------------------------|
| DG              | $Ia\bar{3}d$ (IUC 230) | $m\bar{3}m$ $O_h$       |
| SG/ADG          | $I4_132$ (IUC 214)     | 432 $O$                 |
| strained DG     | Fddd (IUC 70)          | mmm $D_{2h}$            |
| strained SG/ADG | F222 (IUC 22)          | 222 $D_2$               |

**Table 1. Space groups of the relevant structures, without and with shear strain.** Here, DG stands for “double gyroid”, SG for “single gyroid”, and ADG for “asymmetric double gyroid”. The two last ones share the same symmetry, with and without strain. The strain considered here is the shear strain described in the main text, for a generic value  $0 < \theta < \pi/4$ . The Python code used to compute the space groups, based on the open-source library spglib (1), is available in the Supporting Informations.

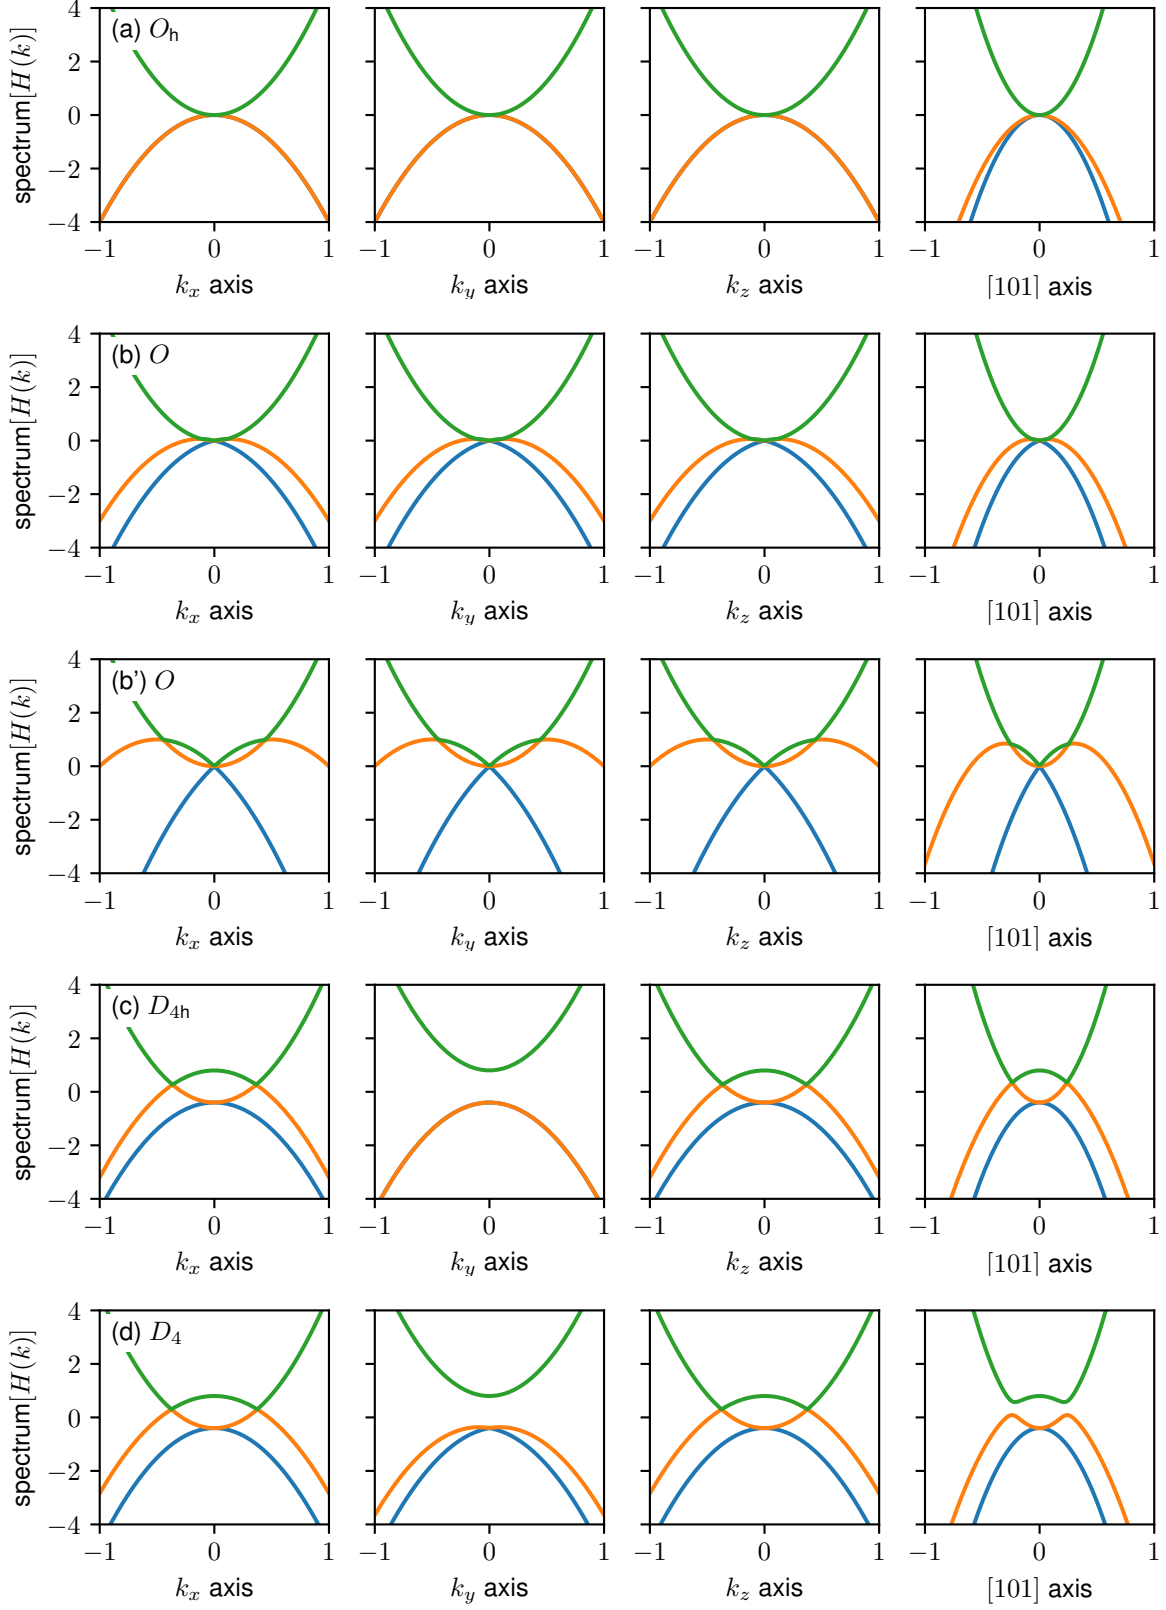

**Fig. 2. Spectra of the effective Hamiltonians for different symmetries.** Spectra of the effective Hamiltonian where the terms from equation 7 of the main text are added to equation 5 of the main text, for different choices of the parameters, corresponding to different point groups at  $\Gamma$ . The spectrum is plotted along the axes which locally correspond to the lines  $\Gamma - H'$ ,  $\Gamma - N'$ ,  $\Gamma - P$ , etc. in the full-wave band structure. (a) The full octahedral symmetry with inversion is present. (b) Inversion symmetry breaking alone [which is exaggerated in (b') for clarity] does modify the relation dispersion, but the three-fold degeneracy at  $\Gamma$  is still present, and the spectrum is still highly symmetric. (c) When inversion is preserved, but that the octahedral group is reduced down to  $D_{4h}$  (or  $D_{2h}$ ), a nodal line opens from the  $\Gamma$  point. (d) This nodal line is split into Weyl points when inversion symmetry is removed, so the point group is  $D_4$  (or  $D_2$ )

group of the wavevector  $\Gamma$  can be obtained from the corresponding point group<sup>\*</sup>, which is isomorphic to  $O_h$ . (For more details on the theory of space groups and their representations, we refer the reader to (8–13).)

We first determine the matrix elements of symmetry operations of the space group  $\mathcal{G}^\Gamma$  of the wavevector  $\Gamma$  in the invariant subspace generated by the set of (orthogonal) degenerate eigenvectors  $\psi_i(\Gamma)$ , with  $i = 1, \dots, g$ , namely by computing

$$[(W, w)]_{ij} = \langle \psi_i(\Gamma) | (W, w) \psi_j(\Gamma) \rangle. \quad [1]$$

Here,  $(W, w) \in \mathcal{G}$  are elements of the space group in Seitz notation, composed of a rotation part described by an operator  $W \in O(d)$  (note that the matrix representing  $W$  is only guaranteed to be orthogonal in a orthonormal basis) and a translation part  $t \in \mathbb{R}^d$ . They compose as  $(W_1, w_1) \cdot (W_2, w_2) = (W_1 W_2, W_1 w_2 + w_1)$ , with inverse  $(W, w)^{-1} = (W^{-1}, -W^{-1}w)$ . The action of the space group on Euclidean points  $x \in \mathbb{E}^d$  is defined by  $(W, w) \cdot x = Wx + w$ . This action on the physical space induces an action on *scalar* functions on this space, defined by  $[(W, w)\phi](x) = \phi((W, w)^{-1}x)$ . The action on a vector field  $\mathcal{E}$  requires to also rotate the components of the vector, and reads

$$[(W, w)\mathcal{E}](x) = W\mathcal{E}((W, w)^{-1}x). \quad [2]$$

In practice, the numerical eigenvectors are obtained as arrays of vectors, representing their amplitude in the discretized primitive unit cell. To compute the rotated eigenvectors, we first linearly interpolate this numerical data with the algorithm of reference (14) as implemented in *scipy* (15), and change the coordinate system into the standard conventional cell. The symmetry operations can be directly extracted from the ITA (3), or e.g. from the Bilbao crystallographic server (4). For each class of symmetries, a representative is applied to the interpolated function through the action defined in equation Eq. (2). The (normalized) overlap is then computed on a discretized grid covering the standard conventional cell. The determinant, trace, etc. of the numerical estimates of the  $g \times g$  overlap matrices  $[(W, w)]$  can then be computed. Our Python implementation is available in the Supporting Materials.

The matrices  $[(W, w)]$  should be unitary. When they are not, the subspace generated by the set of degenerate eigenvectors is actually not left invariant by the action of the symmetries (this may happen e.g. when one eigenvector is singled out of a set of several degenerate eigenvectors). When they are, one can determine which representation  $\Delta$  they form. To do so, one has to compute the character  $\chi_\Delta$  of the representation, i.e. the data of the traces of the overlap matrices for all symmetry operations. As the characters are class functions, it is sufficient to compute the trace of one representative of each symmetry class. Given the characters  $\chi_\Gamma$  or the irreducible representations  $\Gamma$  of the group  $G$  (obtained from its character table; here  $G \simeq O_h$ , see table 2), the representation  $\Delta$  is decomposed by applying the standard Schur reduction formula

$$\langle \chi_\Gamma, \chi_\Delta \rangle = \frac{1}{|G|} \sum_{g \in G} \overline{\chi_\Gamma(g)} \chi_\Delta(g) \quad [3]$$

<sup>\*</sup>The point group of a wavevector  $\mathcal{G}^k$  (also called little co-group at  $k$ ) is the subgroup of the point group  $\mathcal{G}$  associated to the space group  $\mathcal{G}$  of elements which let  $k$  invariant (up to reciprocal lattice vectors). A different (yet related) object is the space group of a wavevector  $\mathcal{G}^k$  (also called little group at  $k$ ), which is the subgroup of the space group of elements whose rotation part leaves  $k$  invariant.

where  $|G|$  is the order of the group, giving the coefficient  $\langle \chi_\Gamma, \chi_\Delta \rangle$  or the irreducible representation  $\Gamma$  in the decomposition of the possibly reducible representation  $\Delta$ . It is convenient to express this coefficient as the sum on the symmetry classes  $[g]$  of the group

$$\langle \chi_\Gamma, \chi_\Delta \rangle = \frac{1}{|G|} \sum_{[g]} n_{[g]} \overline{\chi_\Gamma([g])} \chi_\Delta([g]) \quad [4]$$

where  $n_{[g]}$  is the multiplicity of the class.

| $\overline{m\bar{3}m}$<br>mult. | 1 | 2  | 3  | 4  | 2' | $\bar{1}$ | m  | $\bar{3}$ | $\bar{4}$ | m' |
|---------------------------------|---|----|----|----|----|-----------|----|-----------|-----------|----|
| $A_{1g}$                        | 1 | 1  | 1  | 1  | 1  | 1         | 1  | 1         | 1         | 1  |
| $A_{2g}$                        | 1 | 1  | 1  | -1 | -1 | 1         | 1  | 1         | -1        | -1 |
| $E_g$                           | 2 | 2  | -1 | 0  | 0  | 2         | 2  | -1        | 0         | 0  |
| $T_{1g}$                        | 3 | -1 | 0  | 1  | -1 | 3         | -1 | 0         | 1         | -1 |
| $T_{2g}$                        | 3 | -1 | 0  | -1 | 1  | 3         | -1 | 0         | -1        | 1  |
| $A_{1u}$                        | 1 | 1  | 1  | 1  | 1  | -1        | -1 | -1        | -1        | -1 |
| $A_{2u}$                        | 1 | 1  | 1  | -1 | -1 | -1        | -1 | -1        | 1         | 1  |
| $E_u$                           | 2 | 2  | -1 | 0  | 0  | -2        | -2 | 1         | 0         | 0  |
| $T_{1u}$                        | 3 | -1 | 0  | 1  | -1 | -3        | 1  | 0         | -1        | 1  |
| $T_{2u}$                        | 3 | -1 | 0  | -1 | 1  | -3        | 1  | 0         | 1         | -1 |

**Table 2. Character table of the octahedral group.** Character table of the full octahedral group  $O_h$  ( $m\bar{3}m$ ). Adapted from (16) and (4).

**Photonic double gyroid.** For the three-fold degenerate set composed of the 3<sup>rd</sup>, 4<sup>th</sup>, and 5<sup>th</sup> bands<sup>†</sup>, we find that the electric fields transform along the irreducible representation  $T_{1g}$ , which is indeed three-dimensional. Similarly, for 6<sup>th</sup> band it transforms along the one-dimensional irreducible representation  $A_{2g}$ , while for 7<sup>th</sup> band it transforms along the one-dimensional irreducible representation  $A_{2u}$ , etc. As the magnetic field is a pseudo-vector, it transforms in a different way (17). We can consider the same action Eq. (2) of the space group than for vector field, and one finds that the magnetic fields transform respectively along  $T_{1u}$ ,  $A_{2g}$ , and  $A_{2u}$ . Equivalently, we can modify the action of the space group for pseudo-vector fields as  $[(W, w)\mathcal{H}](x) = \det(W) W\mathcal{H}((W, w)^{-1}x)$  (this simply changes the sign of the transformed field for all improper transformations), in which case the electric and magnetic field transform along the same irreducible representations.

**Dispersive photonic double gyroid.** In the dispersive photonic case, the three-fold degeneracy of interest (at  $\omega/\omega_0 = 0.57$ ) has electric field transforming according to the three-dimensional irreducible representation  $T_{1u}$ . Interestingly, there are also two sets of three-fold degenerate bands above, at  $\omega/\omega_0 = 0.87$  and  $\omega/\omega_0 = 0.92$ , which respectively transform as  $T_{2u}$  and  $T_{2g}$ . The electric field for the next bands transforms according to  $E_g$ ,  $A_{2u}$ , etc. As in the photonic case, we do not consider the zero-frequency zero-momentum eigenvectors, and the behavior of the magnetic field can be obtained from the behavior of the electric field.

<sup>†</sup>We do not consider the 1<sup>st</sup> and the 2<sup>nd</sup> bands: this analysis is not meaningful for the zero-frequency zero-momentum eigenvectors, as the point  $(k, \omega) = (0, 0)$  is singular. Indeed, any uniform field is a solution at this point, while when  $k \neq 0$ , only two independent uniform transverse waves are solutions.

**Phononic double gyroid.** In the phononic double gyroid, we consider the transformation properties of the displacement fields (see the paragraph *Phononic band structures* of the section *Numerical computation of the band structures* of the Supporting Materials), at the center of the Brillouin zone. The three zero-frequency eigenvectors transform according to  $T_{1u}$  (as expected, the family of Cartesian coordinates  $(x, y, z)$  transforming according to  $T_{1u}$ ). At the three-fold degeneracy at  $\omega/\omega_0 \simeq 0.95$ , the eigenvectors transform according to the three-dimensional irreducible representation  $T_{1u}$ , confirming that there is an essential degeneracy. The next two bands transform respectively according to  $A_{2g}$  and  $A_{2u}$ . Near  $\omega/\omega_0 \simeq 1.6$ , there is a surprising feature in the band structure, which resembles a double Dirac cone. While such a feature calls for a more detailed investigation, it is outside of the scope of this paper. The six degenerate eigenvectors involved seem to transform according to  $T_{1g} \oplus T_{1u}$ .

**Effective Hamiltonians from the method of invariants.** Here, the method of invariants (18–22) allows (i) to describe the neighborhood of the three-fold degeneracy involving the 3<sup>rd</sup>, 4<sup>th</sup>, and 5<sup>th</sup> bands of the band structure of the symmetric double gyroid, and (ii) to determine the qualitative effects of symmetry-breaking perturbations of this structure on the frequency bands. The first step consists in determining to which irreducible representation  $\Gamma$  the eigenstates corresponding to the three degenerate bands belong, and to compute the irreducible representation decomposition of  $\Gamma \times \Gamma^*$ . Here, we can skip half of this step (which is however performed in the paragraph *Determination of the irreducible representations at  $\Gamma$*  of the SI to ensure that the representation is irreducible) as all three-dimensional IR of octahedral group  $O_h$  have the same IR decomposition  $\Gamma \times \Gamma^* \simeq A_{1g} + E_g + T_{1g} + T_{2g} = D^X$  ( $\Gamma$  has to be three-dimensional as the degeneracy is three-fold). A set of basis matrices  $X$  for the  $(3 \times 3)$ -dimensional representation  $D^X$  can be chosen as the matrices  $(\text{Id}, L_x, L_y, L_z, \{L_x, L_y\}, \{L_y, L_z\}, \{L_z, L_x\}, \Lambda, \Lambda^\dagger)$  defined in the main text, and are arranged by irreducible representation in table 4, along with irreducible polynomials in  $k_i$  up to third order. The next step is to combine the basis matrices  $X^{\gamma, \mu}$  with the irreducible polynomials  $\mathcal{K}^{\lambda, \mu}$  to form *invariants*, as formulated in equation 4 of the main text. For example, for  $\Gamma_{12} = E_g$ , basis matrices are  $X^{12,1} = \Lambda$ ,  $X^{12,2} = \Lambda^\dagger$ , while irreducible polynomials up to second order are  $\mathcal{K}^{12,1} = K$  and  $\mathcal{K}^{12,2} = \bar{K}$ . Hence, the invariant corresponding to the IR  $\Gamma_{12}$  at second order in  $q$  is

$$\sum_{\mu=1,2} X^{(12,\mu)} \overline{\mathcal{K}^{(12,\mu)}} = \bar{K}\Lambda + K\Lambda^\dagger. \quad [5]$$

The effective Hamiltonian of equation 4 of the main text is obtained by summing all invariants with coefficient such as  $a_\gamma^{(N)}$  (where  $N$  keeps track of the order in  $q$ ), which depend on the details of the system: the symmetry analysis only determines that this coefficient is possibly (and generically) nonzero. In the case of the octahedral group, we obtain the Luttinger Hamiltonian (18) reproduced in equation 5 of the main text.

When the symmetry is lowered, the point group at the relevant  $k$ -point (here  $\Gamma$ ) is reduced to a subgroup. As such, there are fewer constraints, and new combinations of the same irreducible polynomials and basis matrices are allowed in the

effective Hamiltonian (because they are now invariant with respect to the reduced set of symmetries). To find which new terms are allowed, it is convenient to use subduction tables (as in table 3) which relate irreducible representations of a group to the ones of its subgroups. Note that when the descent in symmetry is not trivial (the IRs are not one-dimensional and/or the IR correspondence is not one-to-one), all such combinations may not be invariant, and should either be deduced from the irreducible polynomials and basis matrices of the subgroup, or constrained by direct computation. This procedure yields the new terms in equation 7 of the main text for the group  $D_2$  (for the group  $D_{2h}$ , which is a direct product of  $D_2$  with the group containing only the identity and inversion, one only has to add the additional constraint  $\gamma_i = 0$  due to inversion). Slices of typical spectra of the unperturbed ( $O_h$ -symmetric) and of the perturbed ( $D_{2h}$ -symmetric and  $D_2$ -symmetric) effective Hamiltonians are shown in figure 2.

| $O_h$    | $O$   | $D_{2h}$                   | $D_2$             |
|----------|-------|----------------------------|-------------------|
| $A_{1g}$ | $A_1$ | $A_g$                      | $A$               |
| $A_{2u}$ | $A_2$ | $A_u$                      | $A$               |
| $E_g$    | $E$   | $2A_g$                     | $2A$              |
| $T_{1g}$ | $T_1$ | $B_{1g} + B_{2g} + B_{3g}$ | $B_1 + B_2 + B_3$ |
| $T_{2g}$ | $T_2$ | $B_{1g} + B_{2g} + B_{3g}$ | $B_1 + B_2 + B_3$ |
| $T_{1u}$ | $T_1$ | $B_{1u} + B_{2u} + B_{3u}$ | $B_1 + B_2 + B_3$ |
| $T_{2u}$ | $T_2$ | $B_{1u} + B_{2u} + B_{3u}$ | $B_1 + B_2 + B_3$ |

**Table 3. Descent of symmetry from the octahedral group.** Partial subduction tables from  $O_h$  to  $O$ ,  $D_{2h}$  and  $D_2$ . Only the relevant IR are included. The subduction from  $O_h$  to  $O$  or from  $D_{2h}$  to  $D_2$  simply consists in dropping the gerade/ungerade indices. Adapted from (16).

It may be reassuring to directly check that the effective Hamiltonian is actually invariant under  $O_h$ . It is easy to do so given the representations of the symmetry elements. A set of generators for  $O_h$  is provided by the rotations  $C_4^z \equiv 4_{001}^+$  and  $C_3^{xyz} \equiv 3_{111}^+$  and inversion  $i \equiv \bar{1}$  (23), which are here represented by matrices  $\mathcal{D}(C_4^z) = e^{-i(2\pi/4)L_z}$ ,  $\mathcal{D}(C_3^{xyz}) = e^{-i(2\pi/3)(L_x + L_y + L_z)/\sqrt{3}}$  and  $\mathcal{D}(i) = -\text{Id}_3$ . With Luttinger’s choice of basis matrices, which we follow, time-reversal is represented by complex conjugation alone (remind that while the unitary matrix representing a *unitary* operator transforms as  $\mathcal{O} \mapsto U\mathcal{O}U^{-1}$  through a change of basis, the *unitary* matrix  $\mathcal{A}$  representing an *antiunitary* operator transforms  $\mathcal{A} \mapsto U\mathcal{A}\bar{U}^{-1}$  through the same change of basis), and the Luttinger Hamiltonian is indeed time-reversal invariant.

**Numerical computation of the band structures.** Full-wave computations of the photonic band structures were performed with the open-source package MPB, which determines the fully-vectorial eigenmodes of Maxwell equations with periodic boundary conditions (24). The corresponding control files are available as Supporting Material. To compute the full-wave acoustic, phononic, and dispersive photonic band structures, we developed an efficient finite-difference frequency-domain code based on the parallel Arnoldi package ARPACK (25). This code has been validated in previous studies (26–28), where more details on the implementation can be found.

A technical difficulty comes from the existence of unavoidable discretization artifacts in a BCC FFT grid (29, 30) (interestingly, this issue was identified in photonic crystals based

| Sc.             | (22)           | Bi.          | dim. | even w.r.t time-reversal                                                                     | odd w.r.t time-reversal                                                                                                          |
|-----------------|----------------|--------------|------|----------------------------------------------------------------------------------------------|----------------------------------------------------------------------------------------------------------------------------------|
| A <sub>1g</sub> | $\Gamma_1$     | $\Gamma_1^+$ | 1    | $k^2, \text{Id}$                                                                             | —                                                                                                                                |
| A <sub>2u</sub> | $\Gamma_{2'}$  | $\Gamma_2^-$ | 1    | —                                                                                            | $k_x k_y k_z$                                                                                                                    |
| E <sub>g</sub>  | $\Gamma_{12}$  | $\Gamma_3^+$ | 2    | $(K, \bar{K})$<br>$(\Lambda, \Lambda^\dagger)$                                               | —                                                                                                                                |
| T <sub>1g</sub> | $\Gamma_{15'}$ | $\Gamma_4^+$ | 3    | —                                                                                            | $(L_x, L_y, L_z)$<br>$([k_x, k_y], [k_y, k_z], [k_z, k_x])$                                                                      |
| T <sub>2g</sub> | $\Gamma_{25'}$ | $\Gamma_5^+$ | 3    | $(\{k_x, k_y\}, \{k_y, k_z\}, \{k_z, k_x\})$<br>$(\{L_x, L_y\}, \{L_y, L_z\}, \{L_z, L_x\})$ | —                                                                                                                                |
| T <sub>1u</sub> | $\Gamma_{15}$  | $\Gamma_4^-$ | 3    | —                                                                                            | $(k_x, k_y, k_z)$<br>$(k_x^3, k_y^3, k_z^3)$                                                                                     |
| T <sub>2u</sub> | $\Gamma_{25}$  | $\Gamma_5^-$ | 3    | —                                                                                            | $(k_x(k_y^2 + k_z^2), k_y(k_z^2 + k_x^2), k_z(k_x^2 + k_y^2))$<br>$(k_x(k_y^2 - k_z^2), k_y(k_z^2 - k_x^2), k_z(k_x^2 - k_y^2))$ |

**Table 4. Basis matrices and irreducible polynomials for the octahedral group.** Various notations coexist for the RI: Sc. is the Schoenflies notation, Bi. comes from the Bilbao crystallographic server, and another comes from (22). The curly brackets correspond to symmetric products  $\{A, B\} = (AB + BA)/2$ , while the square brackets are anticommutators  $[A, B] = AB - BA$ . Note that without a magnetic field, the anticommutators of the momentum components like  $[k_x, k_y]$  identically vanish, and should not be considered. Adapted from (22), with elements from (16).

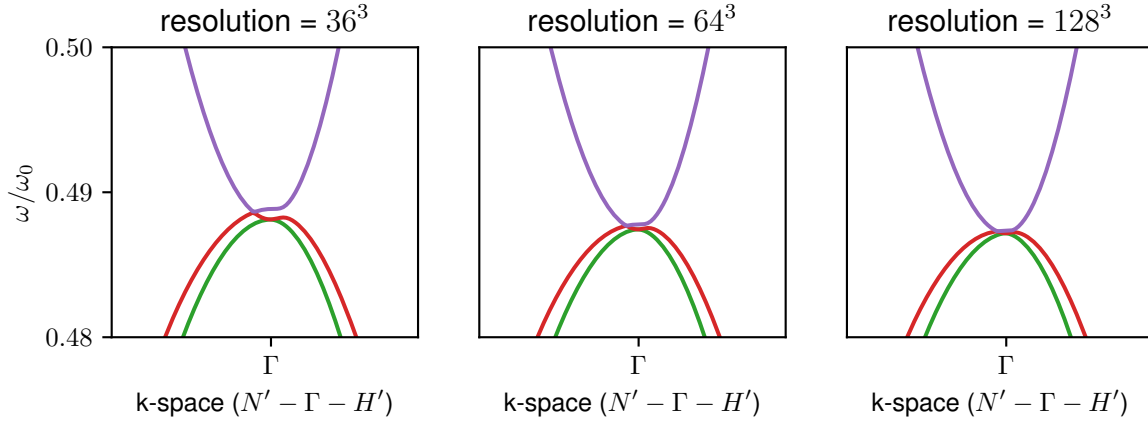

**Fig. 3. Effect of symmetry-breaking numerical errors.** In the structure with asymmetry, but without strain (so the point group at  $\Gamma$  is  $O$ ) We expect that a three-fold degeneracy at  $\Gamma$  should be observed when no strain is applied (whether asymmetry is present or not, see figure 2, (a), (b) and (b')). In the numerical computations however, we observe that even for  $\theta = 0$  (no strain) this degeneracy is lifted by numerical errors. Indeed, the degeneracy is (slowly) recovered when the resolution is increased. Here, parameters are  $\varepsilon_A = 17$ ,  $\varepsilon_B = 15$ ,  $t_A = 1.0$ ,  $t_B = 1.2$ , and the band structure is computed on a  $(n \times 3)^3$  grid with (a)  $n = 36$ , (b)  $n = 64$ , (c)  $n = 128$ .

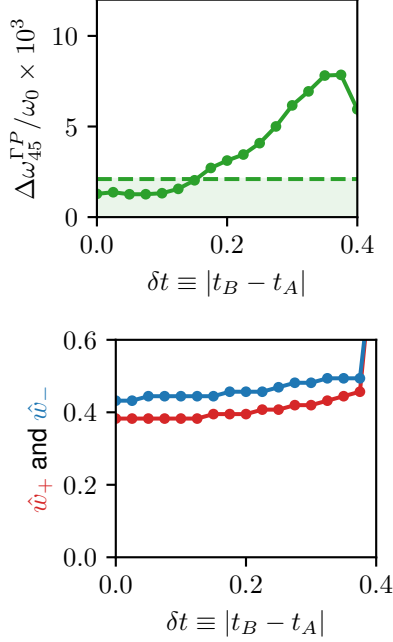

**Fig. 4. Effect of the thickness asymmetry.** Here, the value of the strain angle is fixed to  $\theta = 0.3$  (as in figure 5B of the main text), and there is no asymmetry in the dielectric constants. See figure 5B of the main text for further comments.

on interwoven gyroid nets). This artificial reduction of the symmetry is most noticeable at high-symmetry points (here the  $\Gamma$  point), where a small gap appears between bands which should be degenerate. Here, the effect of the discretization error is equivalent to a spurious small strain, which (slowly) vanishes when the discretization grid is refined (see figure 3 for an example in the case of a photonic band structure). Numerical errors due to the finite grid size are also present far from symmetry points. Even if their effect there is only qualitative and comparatively small, they however constitute the principal source of uncertainty on quantities extracted from the simulations.

**Photonic band structures.** Starting from Maxwell equations (see main text), a second-order differential equation on the magnetic field only can be obtained (31). After a Fourier transform, it leads to the eigenvalue problem (31)

$$\frac{\omega^2}{c^2} \tilde{\mathcal{H}} = \epsilon_{ijk} \epsilon_{klm} (ik_j + \partial_j) \left[ \frac{1}{\epsilon(r)} (ik_\ell + \partial_\ell) [\tilde{\mathcal{H}}] \right] \quad [6]$$

in Bloch space, where  $\tilde{\mathcal{H}}(k, r)$  is periodic with respect to Bravais lattice translations. This equation is then solved by the MPB package, and we refer to (24) for more details.

**Phononic band structures.** The elastic wave equation for an isotropic medium reads (32)

$$\rho \frac{\partial^2 u_i}{\partial t^2} = \partial_j [\rho c_t^2 \partial_j u_i + \partial_i u_j] + \partial_i [\rho (c_\ell^2 - 2c_t^2) \partial_j u_j] \quad [7]$$

where  $u_i$  is the  $i$ th Cartesian component of the displacement field  $u$ ,  $\partial_j = \partial/\partial x^j$ ,  $\rho$  is the medium density, and  $c_\ell$  and  $c_t$  are respectively the longitudinal and transverse speeds of sound

in the medium. After a Fourier transform, equation Eq. (7) becomes

$$\begin{aligned} \omega^2 \tilde{u}_i = & -1/\rho (\partial_j + ik_j) [\rho c_t^2 (\partial_j + ik_j) [\tilde{u}_i] + (\partial_i + ik_i) [\tilde{u}_j]] \\ & -1/\rho (\partial_i + ik_i) [\rho (c_\ell^2 - 2c_t^2) (\partial_j + ik_j) [\tilde{u}_j]] \end{aligned} \quad [8]$$

where  $\tilde{u}(x)$  is spatially periodic with respect to the Bravais lattice translation. Written in this way, the wave equation is an eigenvalue problem, which can be solved numerically by our finite-difference frequency-domain code by discretizing the unit cell. The solutions of the original wave equation Eq. (7) are recovered as  $u(x, t) = \tilde{u}(x) \exp[i(k \cdot x - \omega t)]$ .

**Dispersive photonic band structures.** The dispersive photonic band structures are computed from the formulation of Maxwell equations for dispersive materials as an eigenvalue problem of reference (33), which essentially consists in introducing auxiliary polarization and polarization velocity fields for each Lorentz pole of the permittivity, which describe the dynamics of the corresponding local mechanical oscillators. The dynamics of all coupled fields is then a standard eigenvalue problem. The metallic double gyroid is modeled as a Drude metal, whose frequency-dependent dielectric function is described by a Lorentz pole as

$$\epsilon(\omega) = \epsilon_\infty \left( 1 + \frac{\omega_p^2}{\omega_0^2 - \omega^2 + i\omega\Gamma} \right) \quad [9]$$

where  $\omega_p$  is the plasma pulsation of the metal, and  $\Gamma$  a loss coefficient. In the numerical simulations, the characteristic frequency of the pole is set to  $\omega_0 = 0$ , and  $\epsilon_\infty = 1$ .

**Acoustic band structures.** The acoustic band structures are computed in the same way as phononic band structures, but here the dynamics is governed by the Helmholtz equation

$$\rho \partial_i \left( \frac{1}{\rho} \partial_i p \right) = \frac{\omega^2}{c_\ell^2} p, \quad [10]$$

which is, again, Fourier transformed to take into account the translational invariance, and cast into a matrix eigenvalue problem by discretizing the unit cell.

**Numerical computation of charges of the Weyl points.** We computed the charges of the Weyl points from the numerical Bloch eigenvectors obtained through MPB. To do so, the Bloch eigenvectors were computed on a grid discretizing the surface of a small cube surrounding each Weyl point in the three-dimensional Brillouin zone. On the two-dimensional surface of the cube, a gap separates the two bands involved in the Weyl degeneracy. The charge of the Weyl point can then be related to the first Chern number of the bottom band limited to this surface (they are equal up to a sign), which can in turn be computed from its Berry curvature, defined in terms of the eigenvectors (see below for more details). Numerically, it is convenient to use the gauge-invariant method inspired from lattice gauge theory (34–36) and demonstrated in the context of topological insulators by Fukui, Hatsugai and Suzuki (37) [see also (38–41)]. We implemented this method in Python (the source code is available as Supporting Material). For the convenience of the reader, we review the method in the following.

The topological charge of a Weyl point can be expressed<sup>†</sup> as the opposite of the first Chern number of the band below the gap (the valence band), so the singularity described by the Hamiltonian  $q_i v_{ij} \sigma_j$  has a charge  $\text{sgn det}(v)$ . The first Chern number of an orthogonal projector family  $k \mapsto P(k)$  defined on a two-dimensional manifold  $\mathcal{M}$  can be expressed the normalized integral of the (trace of the) Berry curvature associated to the projected connection  $\nabla^P = P d$  on  $\mathcal{M}$ , namely

$$C_1(P) = \frac{i}{2\pi} \int_{\mathcal{M}} \text{tr} [P dP \wedge dP]. \quad (11)$$

Associated with the projected connection  $\nabla^P$  is a local connection form  $\mathcal{A}$  such that, locally,  $\nabla^P s = (d + \mathcal{A})s$  for any section  $s$  (given a *local* frame  $(e_i(k))_i$ , the components of the connection form may be computed as  $\mathcal{A}_{ij} = \langle e_i, \nabla^P e_j \rangle$ ). The curvature form  $\mathcal{F} = P dP \wedge dP$  is related to the connection form through  $\mathcal{F} = d\mathcal{A} + \mathcal{A} \wedge \mathcal{A}$ . The first Chern number only involves the trace  $F = \text{tr} \mathcal{F}$  of the curvature form, which can be expressed as  $F = dA$  in terms of the trace  $A = \text{tr} \mathcal{A}$  of the connection form. The key feature of a connection is to define a *parallel transport*, where parallel transported sections satisfy  $\nabla^P s \equiv (d + \mathcal{A})s = 0$ . Given an initial condition  $s(0)$  and a path  $\mathcal{C}$  on the base manifold, this differential equation defines a unitary “evolution operator”  $U_{\mathcal{C}}(t)$ , such that  $s(t) = U_{\mathcal{C}}(t)s(0)$  is parallel transported along  $\mathcal{C}$ , which can be expressed as the path-ordered exponential

$$U_{\mathcal{C}}(t) = P \exp \left( - \int_{\mathcal{C}} \mathcal{A} \right). \quad (12)$$

Its trace  $W_{\mathcal{C}}(t) = \text{tr} U_{\mathcal{C}}(t)$  is called a Wilson line, and when the path  $\mathcal{C}$  is closed, the *Wilson loop*  $W_{\mathcal{C}}(1)$  is gauge invariant.

Here, we only need to consider a situation where the frequency band of interest is only composed of one eigenvector at each  $k$  point (or in other words, the vector bundle of interest is of rank one)<sup>§</sup>. Let us denote by  $\psi(k)$  the eigenvector corresponding to the frequency band of interest, corresponding to the orthogonal projector family  $P = |\psi\rangle\langle\psi|$ . The connection form is then  $A = \langle \psi | P d\psi \rangle = \langle \psi | \partial_k \psi \rangle dk$ , and the curvature form is  $F = dA$ . (While  $\psi$  and  $A$  are only defined locally,  $P$  and  $F$  are defined globally.)

To evaluate the first Chern number Eq. (11), one has to resort to numerical diagonalization algorithms, which only determine eigenvectors at each wavevector up to an arbitrary and uncontrollable phase. To overcome this arbitrary phase, discretization should be performed in a gauge-invariant way. First, the manifold  $\mathcal{M}$  is discretized into a polygon mesh  $\tilde{\mathcal{M}}$ . As the curvature  $F$  is gauge invariant, so is its integral over any surface. Hence, for a sufficiently fine mesh, the integral Eq. (11) is well-approximated by the sum of integrals

$$C_1(P) \approx \frac{i}{2\pi} \sum_{p \in \tilde{\mathcal{M}}} \int_p F, \quad (13)$$

where the sum runs on all polygons  $p$  of the mesh  $\tilde{\mathcal{M}}$ . Each surface integral can be transformed into a line integral on its

boundary through Stokes theorem, as

$$\int_p F = \int_{\partial p} A = \sum_{e \subset p} \int_e A \quad (14)$$

where  $e \subset p$  are the edges of the polygon  $p$ . As the connection is defined as

$$A(k) = \lim_{q \rightarrow 0} \frac{1}{q} \langle \psi(k) | \psi(k+q) - \psi(k) \rangle \quad (15)$$

it can also be expressed as

$$A(k) = \frac{\partial}{\partial q} \left[ \log \frac{\langle \psi(k) | \psi(k+q) \rangle}{|\langle \psi(k) | \psi(k+q) \rangle|} \right]. \quad (16)$$

This expression is particularly useful as it allows to approximate the line integral of  $A$  over a small line as the logarithm of a discretized Wilson line. In turn, the line integral on a closed curve will be approximated as a discrete Wilson loop. An edge  $e = [v_1, v_2]$  is a segment going from the vertex  $v_1$  to the vertex  $v_2$  (which obviously depend on  $e$ !), so its boundary is  $\partial e = [v_2] - [v_1]$ . The integral over such an edge is then approximated as

$$\int_{e \equiv [v_1, v_2]} A \approx \log \frac{\langle \psi(v_1) | \psi(v_2) \rangle}{|\langle \psi(v_1) | \psi(v_2) \rangle|}. \quad (17)$$

This expression is indeed not gauge invariant. However, the integral over the closed path  $\partial p$  can be written as

$$\int_{\partial p} A = \log \left[ \prod_{e \equiv [v_1, v_2] \subset p} \frac{\langle \psi(v_1) | \psi(v_2) \rangle}{|\langle \psi(v_1) | \psi(v_2) \rangle|} \right]. \quad (18)$$

As the  $\partial p$  is a closed loop, all vertices appear exactly two times in this product (one as a bra, one as a ket), which gets rid of all arbitrary phases. For example, if  $p = [k_1, k_2, k_3]$  is a triangle, then Eq. (18) becomes

$$\log \left[ \frac{\langle \psi(k_1) | \psi(k_2) \rangle}{|\langle \psi(k_1) | \psi(k_2) \rangle|} \frac{\langle \psi(k_2) | \psi(k_3) \rangle}{|\langle \psi(k_2) | \psi(k_3) \rangle|} \frac{\langle \psi(k_3) | \psi(k_1) \rangle}{|\langle \psi(k_3) | \psi(k_1) \rangle|} \right]. \quad (19)$$

Finally, the first Chern number is expressed as

$$C_1(P) \approx \frac{i}{2\pi} \sum_{p \in \tilde{\mathcal{M}}} \log \left[ \prod_{e \equiv [v_1, v_2] \subset p} \frac{\langle \psi(v_1) | \psi(v_2) \rangle}{|\langle \psi(v_1) | \psi(v_2) \rangle|} \right]. \quad (20)$$

Note that the polygon mesh and its polygons inherit the orientation of the manifold  $\mathcal{M}$ , and in turn determine the orientation of the boundaries  $\partial p$  and of the edges  $e$ .

Concretely, we find in the case at hand (same parameters as in figure 4 of the main text, with a  $(32 \times 3)^3$  grid for the unit cell) that the first Chern number of the 4<sup>th</sup> band on a cube of length 0.2, centered around the degeneracy on the  $\Gamma - H'$ , with faces discretized by  $10 \times 10$  grids, is  $C_1(W_{\Gamma-H'}, 4^{\text{th}}) = -1$ . The same computation for the degeneracy on the  $\Gamma - N'$  line yields  $C_1(W_{\Gamma-N'}, 4^{\text{th}}) = 1$ . In other words, the Weyl point on the  $\Gamma - H'$  line has charge +1 while the Weyl point on the  $\Gamma - N'$  line has charge -1.

The uncertainty on the numerically computed Chern numbers is hard to evaluate, and even to define. Instead, one has to ensure that the mesh discretizing the manifold is fine enough that the absolute value of the discretized Wilson loop  $W(p)$  defined by equation Eq. (18) is smaller than  $\pi$  for all polygons in the mesh (37), namely  $\max_p |W(p)| < \pi$ . Here, we indeed check that  $\max_p |W(p)| \approx 0.70 < \pi$  (on  $\Gamma - H'$ ) and  $\max_p |W(p)| \approx 0.76 < \pi$  (on  $\Gamma - N'$ ).

<sup>†</sup>This expression turns out to be more general than the expression in terms of the velocity matrix, as it also works for so-called *multi-Weyl* points. As such, it should be adopted as the definition of the charge of a Weyl point, while the expression  $\text{sgn det}(v)$  should be viewed as a consequence of this definition in a particular case.

<sup>§</sup>It is worth mentioning that the method can also be used in the non-Abelian case (36, 37, 41).

## Additional informations.

**Geometry of the structure.** As sinusoidal functions are periodic, the system can be obtained by repeating the cubic cell defined by the unit vectors  $u_x = (1, 0, 0)$ ,  $u_y = (0, 1, 0)$  and  $u_z = (0, 0, 1)$ . This conventional cell is however not fundamental; instead, we use the BCC unit cell defined by lattice vectors  $a_1 = (-1, 1, 1)/2$ ,  $a_2 = (1, -1, 1)/2$ ,  $a_3 = (1, 1, -1)/2$ . Without strain, the first Brillouin zone of both the symmetric and asymmetric double gyroid structures is a rhombic dodecahedron (see figure 2 of the main text), whose relevant high-symmetry points are (in the basis of reciprocal lattice vectors  $a_i^*$  such that  $\langle a_i^*, a_j \rangle = 2\pi\delta_{ij}$ ),  $\Gamma = (0, 0, 0)$ ,  $H' = (1/2, 1/2, -1/2)$ ,  $N' = (1/2, -1/2, 0)$ ,  $H = (1/2, -1/2, 1/2)$ , and  $P = (3/4, -1/4, -1/4)$ . When strain is applied, the new lattice vectors are  $\tilde{a}_i = \epsilon a_i$ . The first Brillouin zone is deformed in a possibly complicated way, as depicted in figure 5. To make the comparison easier, we used the same k-path for the strained and unstrained structures, but it should be noted that while in the case of the shear strain used in the main text,  $H'$  and  $N'$  remain high symmetry points, it is not the case for  $H$  nor  $P$ , that leave the first Brillouin zone boundary. However, the  $\Gamma - P$  line remains in the plane spanned by  $\Gamma - H'$  and  $\Gamma - N'$ , so the gap on this line is an acceptable observable to set apart a nodal line from a potential set of Weyl points from the band structure only.

**Uniaxial strain.** Another way to deform the structure consists in applying uniaxial strain  $\epsilon = \text{diag}(1, 1, \epsilon_{zz})$ . In this case, the space group of the asymmetric double gyroid is  $I4_122$  (IUC 98), and the point group at  $\Gamma$  is 422 (i.e.  $D_4$ ). In this case, all the discussion concerning the effective Hamiltonian still applies, with the additional constraints  $g_x = g_y$ ,  $\beta_- = -\sqrt{3}\beta_+$ ,  $\delta_- = -\sqrt{3}\delta_+$ ,  $\zeta_- = -\sqrt{3}\zeta_+$ , and Weyl points are also predicted to appear in this situation.

**Allowed values of the parameters.** As we start from  $t_A = t_B = \bar{t} = 1.1$ , the parameter  $\delta t \equiv t_B - t_A$  is constrained to  $|\delta t| \leq 2(\sqrt{2} - \bar{t}) \approx 0.62$  for the structure to exist (and in practice, values very close to the limit may not be reachable). Similarly, the strain angle is constrained to  $0 \leq \theta \leq \pi/4$ , and values close to  $\pi/4$  are not realistic, and starting from  $\epsilon_A = \epsilon_B = \bar{\epsilon} = 16$ ,  $\delta\epsilon \equiv \epsilon_B - \epsilon_A$  is constrained to  $|\delta\epsilon| \leq 2\bar{\epsilon} = 32$ .

**Additional band structures.** The full band structures (starting at zero frequency) of the unperturbed dispersive photonic, phononic, and acoustic systems are provided in figures 8, 9 and 10. The full band structure of the photonic system with different strain angles is provided in figure 7. An interesting case where a Weyl point is spectrally isolated from the other bulk bands is shown in figure 12.

1. Togo A (2017) Spglib. Available at <https://atztogo.github.io/spglib/>.
2. Schoen AH (1970) Infinite periodic minimal surfaces without self-intersections, (NASA Electronics Research Center), Technical Report NASA-TN-D-5541, C-98.
3. Aroyo MI, ed. (2016) *International Tables for Crystallography*. (International Union of Crystallography).

4. Aroyo MI, et al. (2006) Bilbao Crystallographic Server: I. Databases and crystallographic computing programs. *Zeitschrift für Kristallographie - Crystalline Materials* 221(1).
5. Lu L, Fu L, Joannopoulos JD, Soljačić M (2013) Weyl points and line nodes in gyroid photonic crystals. *Nature Photonics* 7(4):294–299.
6. Lu L, et al. (2015) Experimental observation of Weyl points. *Science* 349(6248):622–624.
7. Wang L, Jian SK, Yao H (2016) Topological photonic crystal with equifrequency Weyl points. *Physical Review A* 93(6).
8. Inui Y, Tanabe T, Onodera Y (1990) *Group Theory and Its Applications in Physics*. (Springer).
9. Dresselhaus MS, Dresselhaus G, Jorio A (2008) *Group Theory: Application to the Physics of Condensed Matter*. (Springer), 2008 edition.
10. Bradley C, Cracknell A (2010) *The Mathematical Theory of Symmetry in Solids: Representation Theory for Point Groups and Space Groups*. (Oxford University Press).
11. Tinkham M (1964) *Group Theory and Quantum Mechanics (Dover Books on Chemistry)*. (Dover Publications).
12. Heine V (1960) *Group Theory in Quantum Mechanics: An Introduction to Its Present Usage*. (Dover Publications).
13. Knox RS, Gold A (1964) *Symmetry In The Solid State*. (W. A. Benjamin).
14. Weiser A, Zaranonello SE (1988) A note on piecewise linear and multilinear table interpolation in many dimensions. *Mathematics of Computation* 50(181):189–189.
15. Jones E, Oliphant T, Peterson P, et al. (2001–) SciPy: Open source scientific tools for Python.
16. Altmann SL, Herzog P (1994) *Point-Group Theory Tables*. (Clarendon Press, Oxford).
17. Sakoda K (2004) *Optical Properties of Photonic Crystals*. (Springer), 2nd edition.
18. Luttinger JM (1956) Quantum Theory of Cyclotron Resonance in Semiconductors: General Theory. *Physical Review* 102(4):1030–1041.
19. Pikus GE (1961) A New Method of Calculating the Energy Spectrum of Carriers in Semiconductors. II. Account of Spin-orbit Interaction. *Soviet Physics JETP* 14(5).
20. Bir GL, Pikus GE (1975) *Symmetry and Strain-Induced Effects in Semiconductors*. (IPST).
21. Winkler R (2003) *Spin-Orbit Coupling Effects in Two-Dimensional Electron and Hole Systems*. (Springer Berlin Heidelberg).
22. Willatzen M, Voon LCLY (2009) *The k-p Method*. (Springer Nature).
23. McWeeny R, Jones H (1963) *Symmetry: An Introduction to Group Theory and Its Applications (Dover Books on Physics)*. (Pergamon Press).
24. Johnson S, Joannopoulos J (2001) "Block-iterative frequency-domain methods for Maxwell's equations in a planewave basis". *Optics Express* 8(3):173.
25. Lehoucq RB, Sorensen DC, Yang C (1998) *ARPACK Users' Guide*. (Society for Industrial and Applied Mathematics).
26. Hur K, et al. (2011) Three-Dimensionally Isotropic Negative Refractive Index Materials from Block Copolymer Self-Assembled Chiral Gyroid Networks. *Angewandte Chemie International Edition* 50(50):11985–11989.
27. Jeon SY, Kwon H, Hur K (2017) Intrinsic photonic wave localization in a three-dimensional icosahedral quasicrystal. *Nature Physics* 13(4):363–368.
28. Hur K, Hennig RG, Wiesner U (2017) Exploring Periodic Bicontinuous Cubic Network Structures with Complete Phononic Bandgaps. *The Journal of Physical Chemistry C* 121(40):22347–22352.
29. Saba M, Turner MD, Mecke K, Gu M, Schröder-Turk GE (2013) Group theory of circular-polarization effects in chiral photonic crystals with four-fold rotation axes applied to the eight-fold intergrowth of gyroid nets. *Physical Review B* 88(24).
30. Saba M, Schröder-Turk G (2015) Bloch Modes and Evanescent Modes of Photonic Crystals: Weak Form Solutions Based on Accurate Interface Triangulation. *Crystals* 5(1):14–44.
31. John D, Joannopoulos, Steven G, Johnson JNW, Meade RD (2008) *Photonic Crystals: Molding the Flow of Light*. (Princeton University Press), 2 edition.
32. Achenbach J (1987) *Wave Propagation in Elastic Solids*. (North Holland), 1 edition.
33. Raman A, Fan S (2010) Photonic Band Structure of Dispersive Metamaterials Formulated as a Hermitian Eigenvalue Problem. *Physical Review Letters* 104(8).
34. Lüscher M (1982) Topology of lattice gauge fields. *Communications in Mathematical Physics* 85(1):39–48.
35. Panagiotakopoulos C (1985) Topology of 2D lattice gauge fields. *Nuclear Physics B* 251:61–76.
36. Phillips AV, Stone DA (1990) The computation of characteristic classes of lattice gauge fields. *Communications in Mathematical Physics* 131(2):255–282.
37. Fukui T, Hatsugai Y, Suzuki H (2005) Chern Numbers in Discretized Brillouin Zone: Efficient Method of Computing (Spin) Hall Conductances. *Journal of the Physical Society of Japan* 74(6):1674–1677.
38. King-Smith RD, Vanderbilt D (1993) Theory of polarization of crystalline solids. *Physical Review B* 47(3):1651–1654.
39. Simon R, Mukunda N (1993) Bargmann invariant and the geometry of the Güoy effect. *Physical Review Letters* 70(7):880–883.
40. Resta R (1994) Macroscopic polarization in crystalline dielectrics: the geometric phase approach. *Reviews of Modern Physics* 66(3):899–915.
41. Leone R (2011) The geometry of (non-)Abelian adiabatic pumping. *Journal of Physics A: Mathematical and Theoretical* 44(29):295301.

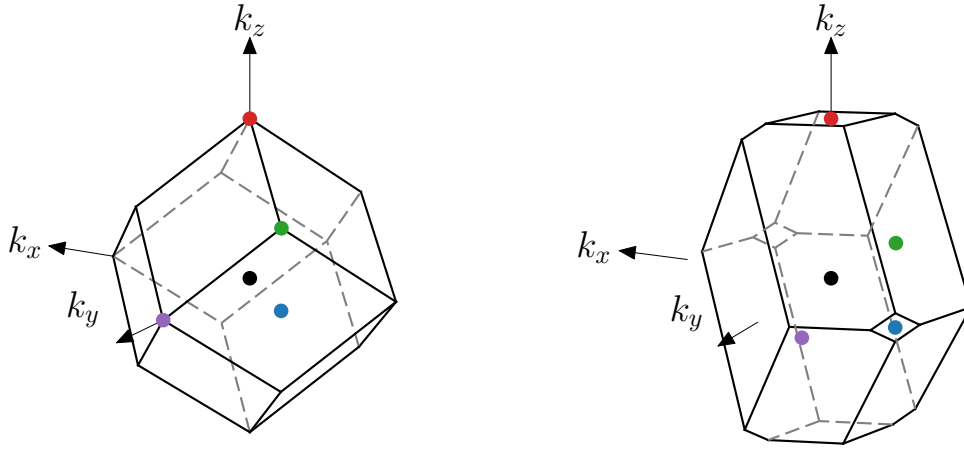

**Fig. 5. Comparison of the first Brillouin zones of the unstrained and the strained structures.** In the strained case (right), the strain angle is  $\theta = 0.3$ . The point  $\Gamma$  is in black,  $H'$  is in red,  $N'$  in blue,  $H$  in purple and  $P$  in green.

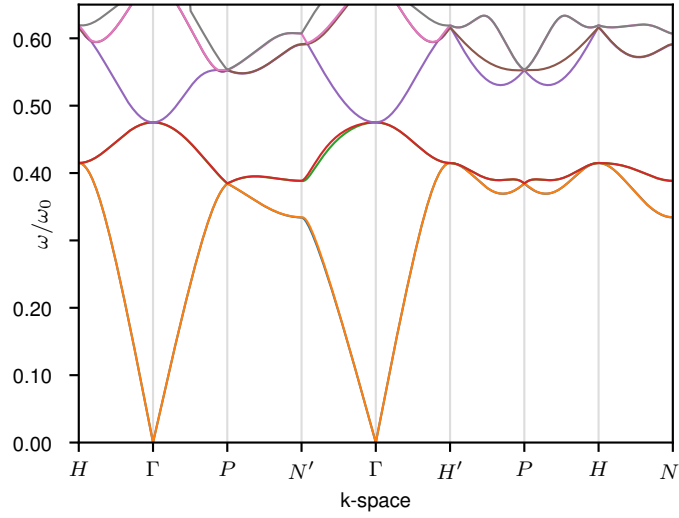

**Fig. 6. Band structure of the unperturbed double gyroid.** This is an unzoned version of figure 4A of the main text.

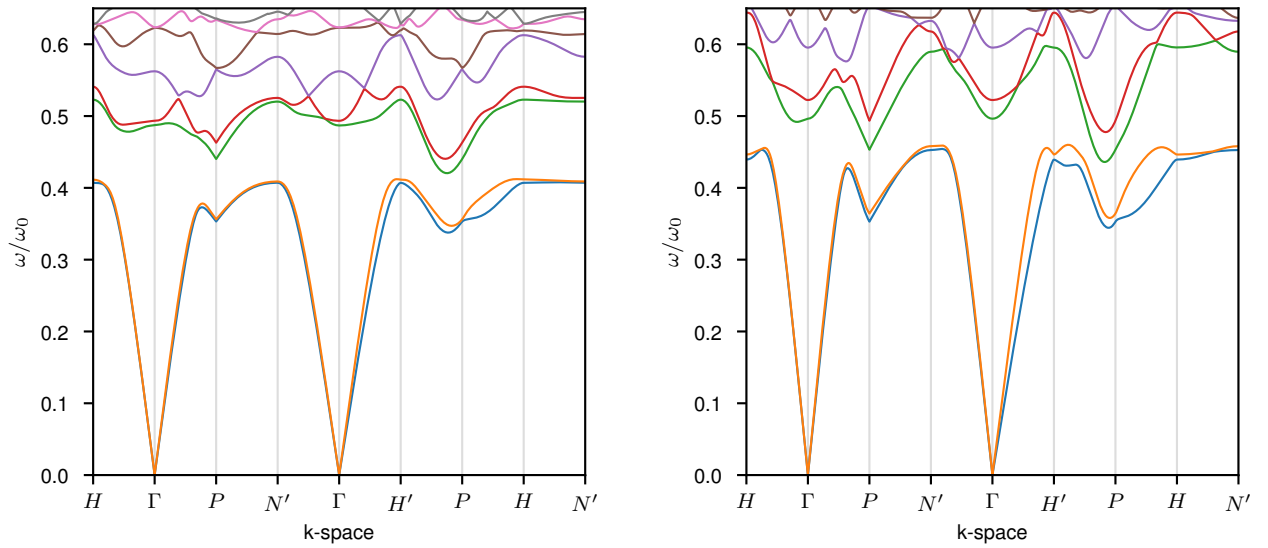

**Fig. 7. Band structure at different strain angles.** The strain angles are  $\theta = 0.3$  (left, which is an unzoned version of figure 4B of the main text) and  $\theta = 0.4$  (right). Other parameters are found in figure 4 of the main text, but the computation is done on a  $(32 \times 3)^3$  grid.

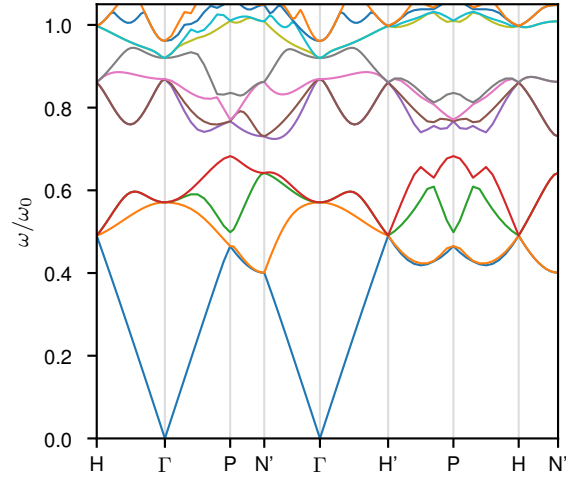

**Fig. 8. Dispersive photonic band structure of the unperturbed double gyroid** The figure 6A of the main text is a zoom of this figure. See its caption for details.

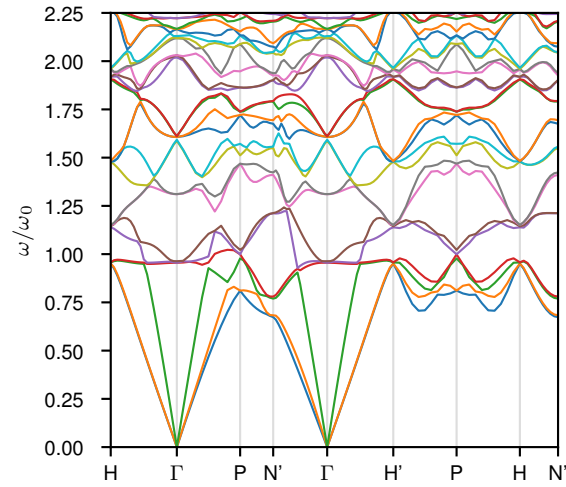

**Fig. 9. Phononic band structure of the unperturbed double gyroid** The figure 6B of the main text is a zoom of this figure. See its caption for details.

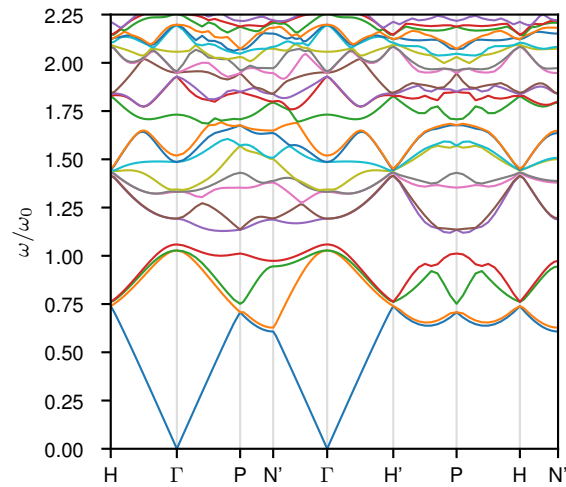

**Fig. 10. Acoustic band structure of the unperturbed double gyroid** The figure 6C of the main text is a zoom of this figure. See its caption for details.

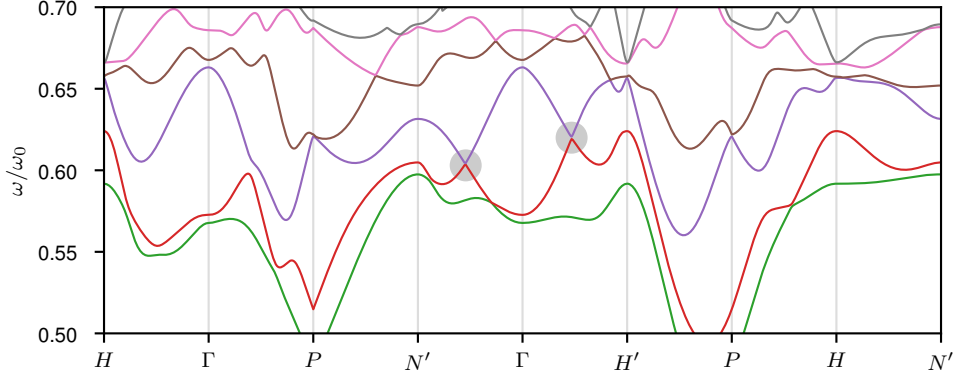

**Fig. 11. Weyl points with lower dielectric contrast.** It is also possible to obtain Weyl points with an asymmetry only in the gyroids' thicknesses, here shown with a lower dielectric contrast 12:1 than in the analysis of the main text and than the one used in figure 4. While the bulk bands overlap then in frequency, Weyl points are still clearly seen on the  $\Gamma - N'$  and  $\Gamma - H'$  lines. Here,  $\varepsilon_A = 12$ ,  $\varepsilon_B = 12$ ,  $t_A = 0.95$ ,  $t_B = 1.25$ , and  $\theta = 0.3$ . The band structure is computed on a  $(32 \times 4)^3$  grid.

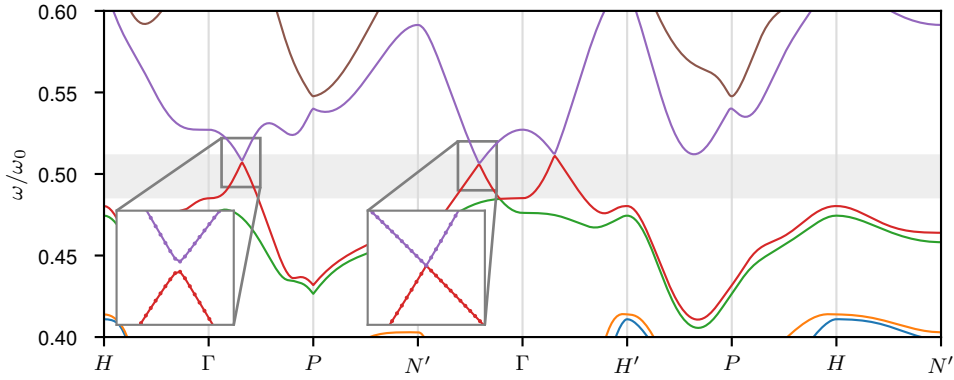

**Fig. 12. Spectrally isolated Weyl point.** We show a zoom on the photonic band structure with slightly different parameters than in figure 4B of the main text. Here, the frequency overlaps with the bulk bands (e.g. on the  $\Gamma - H$  and  $H' - P - H - N'$ ) are significantly removed. The gray band represents the band width available for the Weyl points and the (gapped) nodal line. While the Weyl point on  $\Gamma - H'$  is at the same frequency that the bottom of the purple band on  $H' - P$ , the Weyl point on  $\Gamma - N'$  is not hidden by any bulk band. However, the gap of the gapped nodal line (here on  $\Gamma - P$ ) is very small. This is because the same parameter, the strain angle, is mainly responsible for the opening of the gap on the nodal line and the up and down motion of the bulk bands away from the nodal line: with a more general strain, a frequency isolated Weyl point with a strongly gapped nodal line would be achievable. Here,  $\varepsilon_A = 18.5$ ,  $\varepsilon_B = 13.5$ ,  $t_A = t_B = 1.1$ , and  $\theta = 0.23$ . The main band structure is computed on a  $(32 \times 4)^3$  grid, while the insets are computed on a  $(128 \times 4)^3$  grid, and with a higher resolution in k-space.
